# Supplementary material for: Deep learning assisted SERS detection of prolines and hydroxylated prolines using nitrilotriacetic acid functionalized gold nanopillars
Source: arXiv:2412.08239 source file (2024-12-11)
Supplement: Supplementary file 1 [file Supporting_Information.pdf]

# Supporting information

# Deep learning assisted SERS detection of prolines and hydroxylated prolines using nitrilotriacetic acid functionalized gold nanopillars

**Yuan Zhang [a], Kuo Zhan [a,b], Peilin Xin [a,b], Yingqi Zhao [a,b], Shubo Wang [d], Aliaksandr Hubarevich [e], Xuejin Zhang [f], Jianan Huang [a,b,c,*]**

[a] *Research Unit of Health Sciences and Technology (HST), Faculty of Medicine, University of Oulu, Oulu 90220, Finland.*

[b] *Biocenter Oulu, University of Oulu, Oulu 90220, Finland.*

[c] *Research Unit of Disease Networks, Faculty of Biochemistry and Molecular Medicine, University of Oulu, Oulu 90220, Finland.*

[d] *Nano and Molecular Systems Research Unit, Faculty of Science, University of Oulu, Oulu 90570, Finland.*

[e] *Plasmon Nanotechology Unit, Istituto Italiano di Tecnologia, Via Morego 30, 16163 Genova, Italy*

[f] *School of Physics and College of Engineering and Applied Sciences, Nanjing University, Nanjing 210093, China*

** Corresponding author. Email: jianan.huang@oulu.fi*

**Table of Contents**


1. **Supplementary Figures**

   Figure S1. The reflectance spectra of gold nanopillars.

   Figure S2. The SEM images of Au nanopillars.

   Figure S3. Raman spectra of Au nanopillars and Au-Pro.

   Figure S4. Raman spectrum of solid NTA powder

   Figure S5. Some SERS spectra of Au-NTA

   Figure S6. Some SERS spectra of Au-NTA-Ni-Pro

   Figure S7. Some SERS spectra of Au-NTA-Ni-Hyp

   Figure S8. XPS spectrum of Au-NTA-Ni-Hyp

   Figure S9. XPS spectrum of Au-NTA-Ni-Hyp

   Figure S10. Machine learning figures for Pro and Hyp distinguished train data.

   Figure S11. Distribution histograms of the peak frequency for Au-NTA.

2. **Supplementary Tables**

   Table S1. Peaks assignments of NTA powder and Au-NTA

   Table S2. Peaks assignments of Au-NTA-Ni-Pro and Au-NTA-Ni-Hyp

# 1. Supplementary Figures

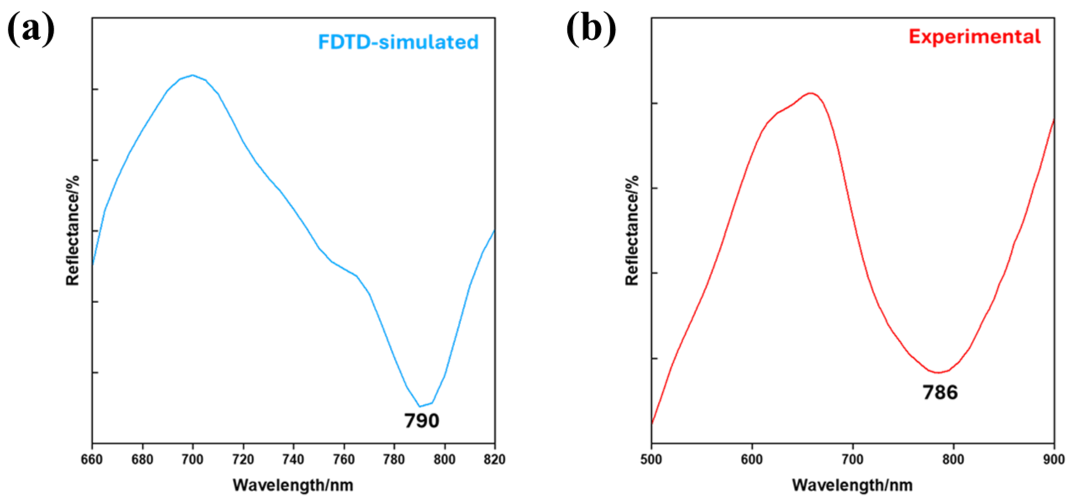


**Figure S1.** The reflectance spectra of gold nanopillars. (a) FDTD-simulated reflectance. (b) The experimental reflectance.

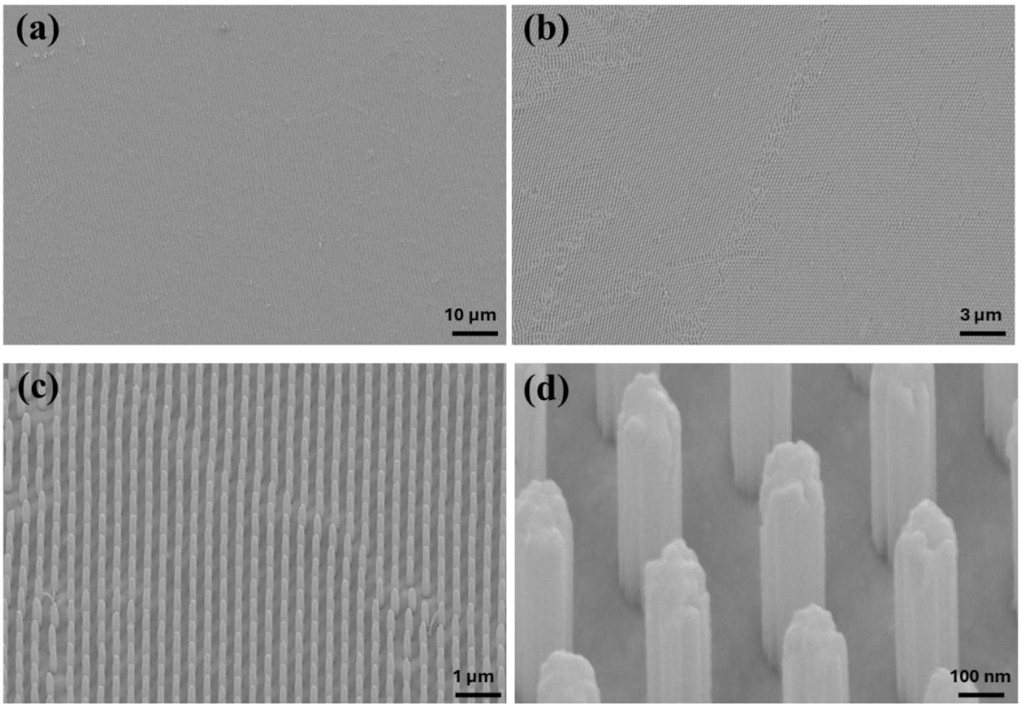


**Figure S2.** The SEM images of Au nanopillars.

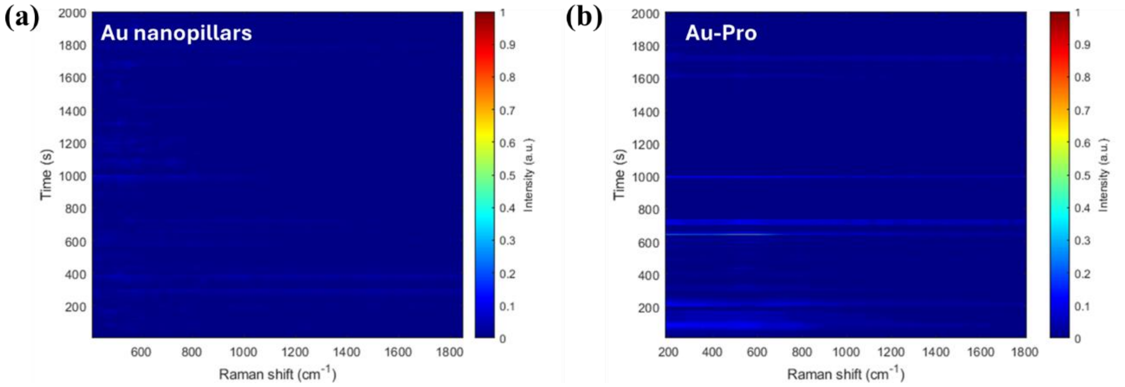


**Figure S3.** Time-series Raman spectra of Au nanopillars (a) and Au nanopillars with Pro (b).

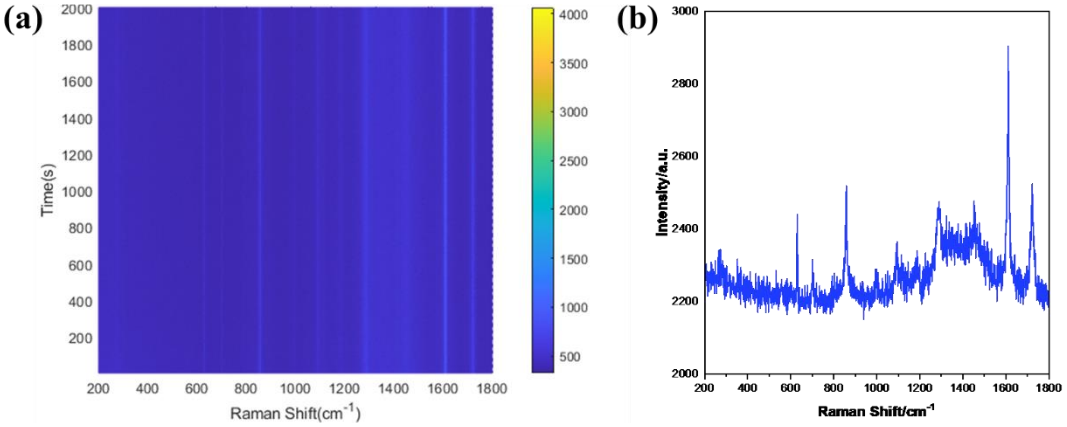


**Figure S4.** Raman spectra of solid NTA powder. (a) Time-series Raman spectrum. (b) The extracted Raman spectra at 1000s.

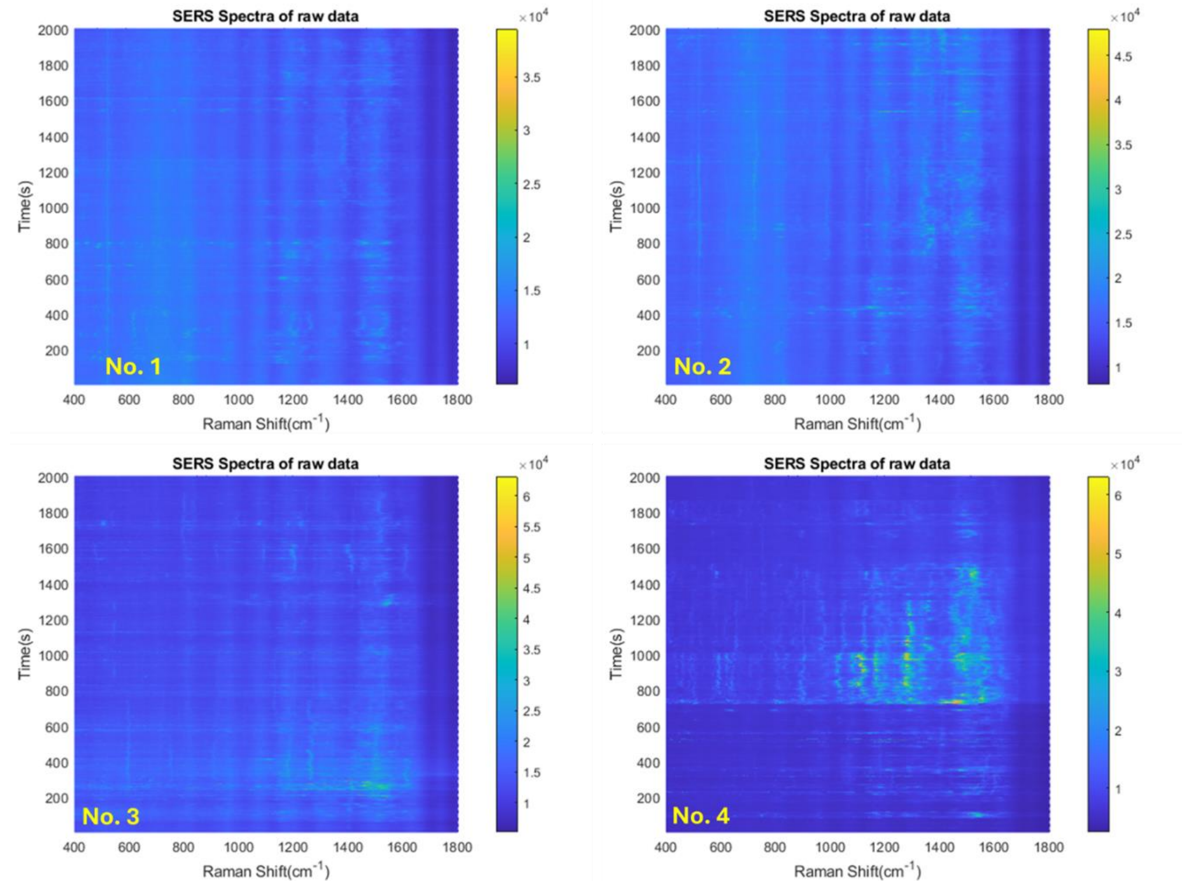


**Figure S5.** Some SERS spectra of Au-NTA.

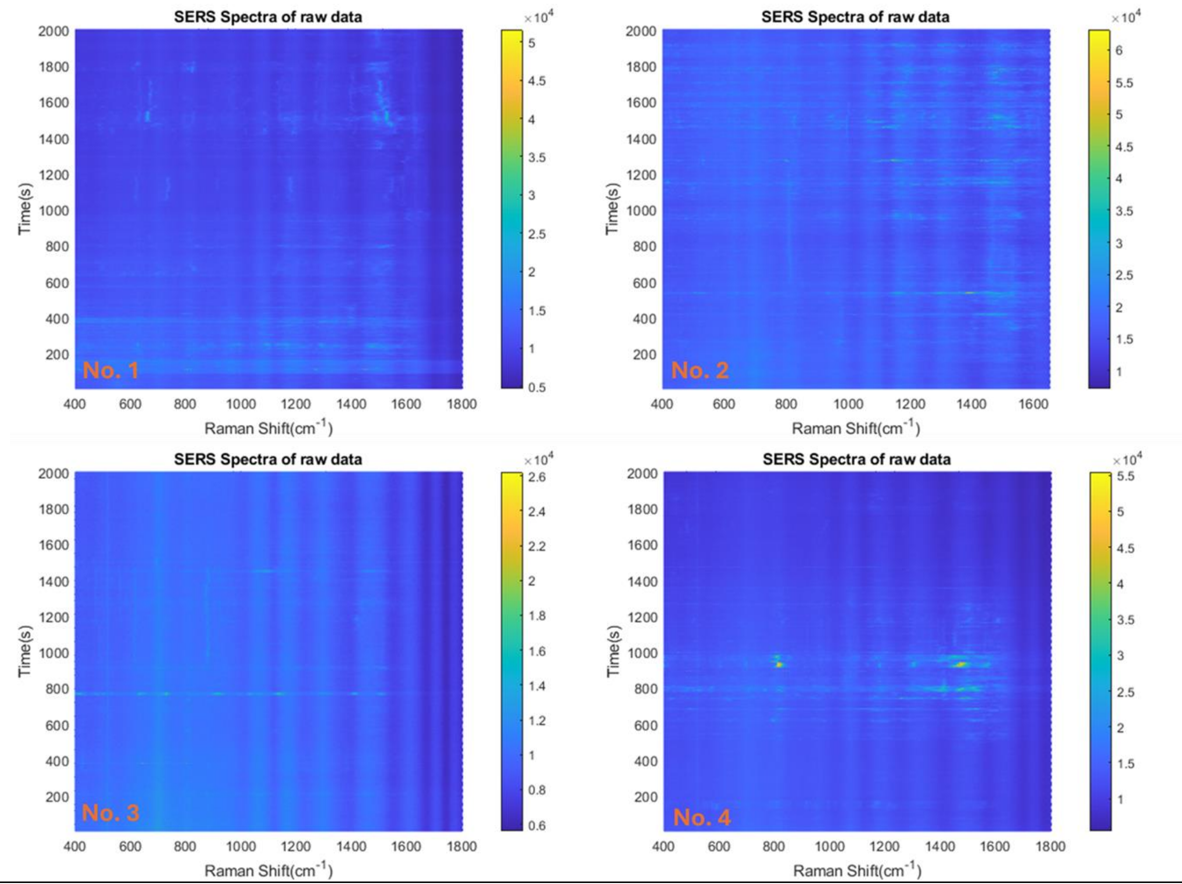

**Figure S6.** Some SERS spectra of Au-NTA-Ni-Pro.

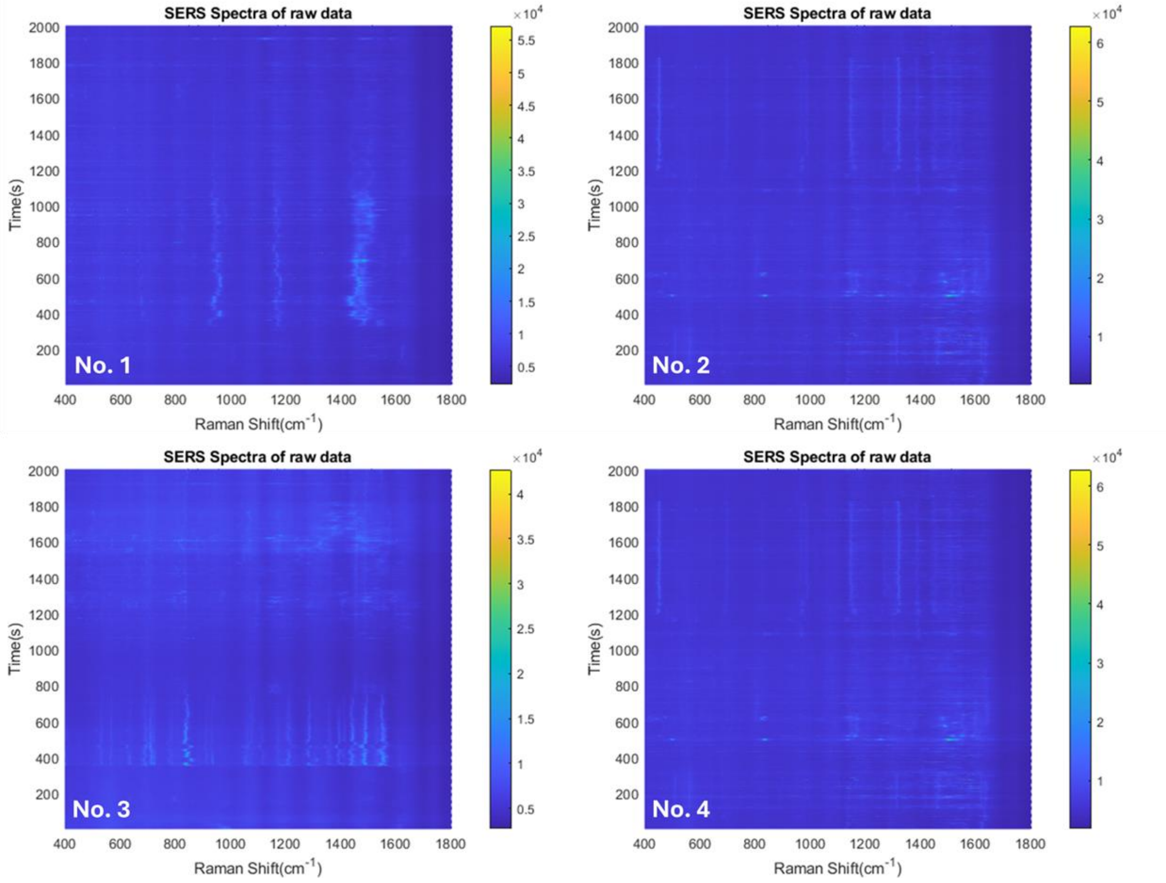


**Figure S7.** Some SERS spectra of Au-NTA-Ni-Hyp.

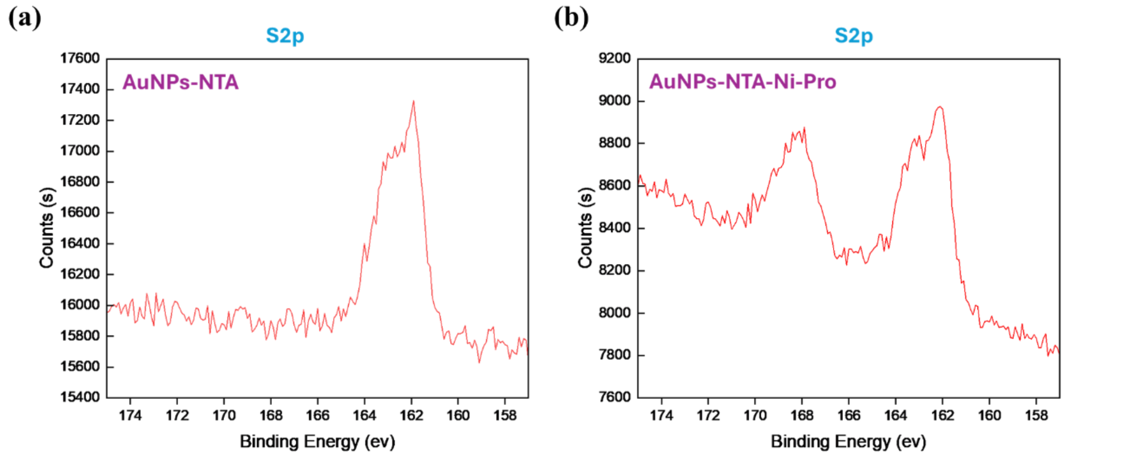


**Figure S8.** XPS spectra of S2p core levels of AuNPs-NTA (a) and AuNPs-NTA-Ni-Pro (b).

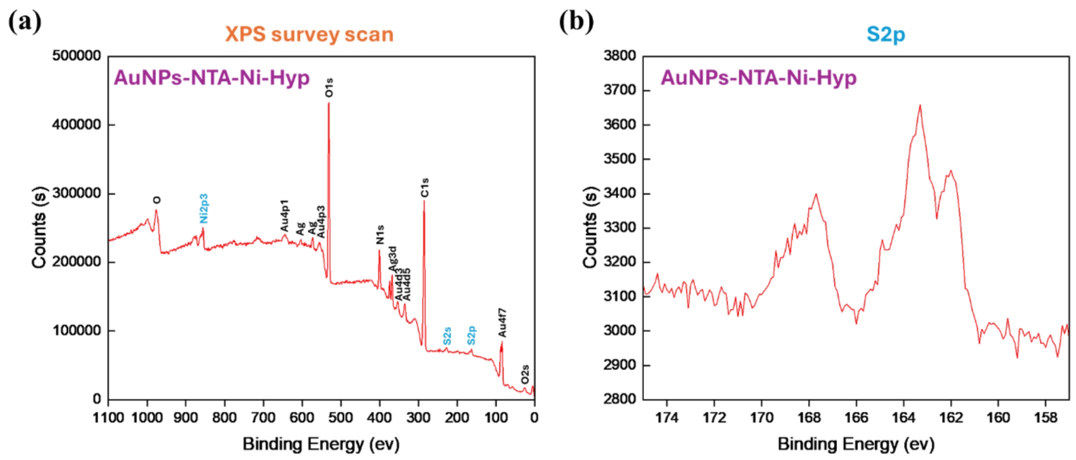


**Figure S9.** XPS results of AuNPs-NTA-Ni-Hyp. (a) XPS survey scan of AuNPs-NTA-Ni-Hyp. (b, c) High-resolution XPS spectra for S 2p (b) and Ni 2p (c) core level.

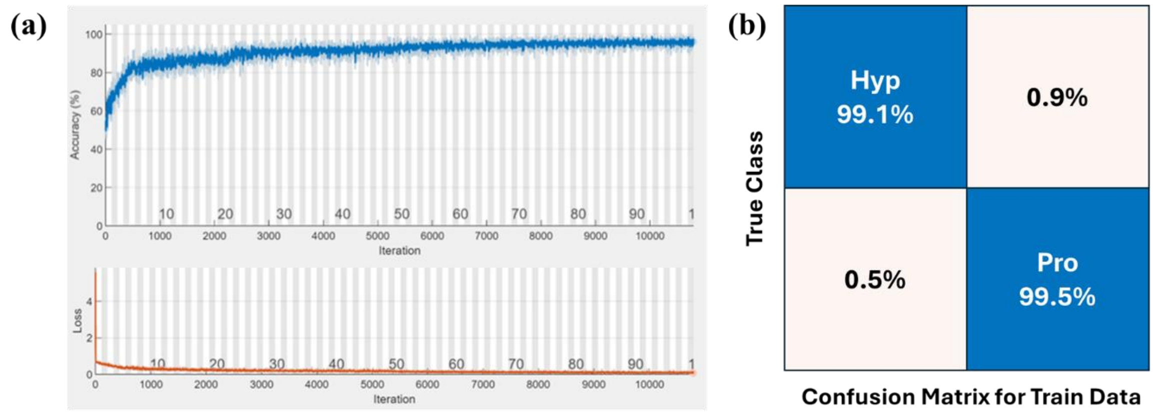


**Figure S10.** Machine learning figures for Au-NTA-Ni-Pro and Au-NTA-Ni-Hyp distinguished train data. (a) The loss and accuracy curve results of train data. (b) The accuracy of train data.

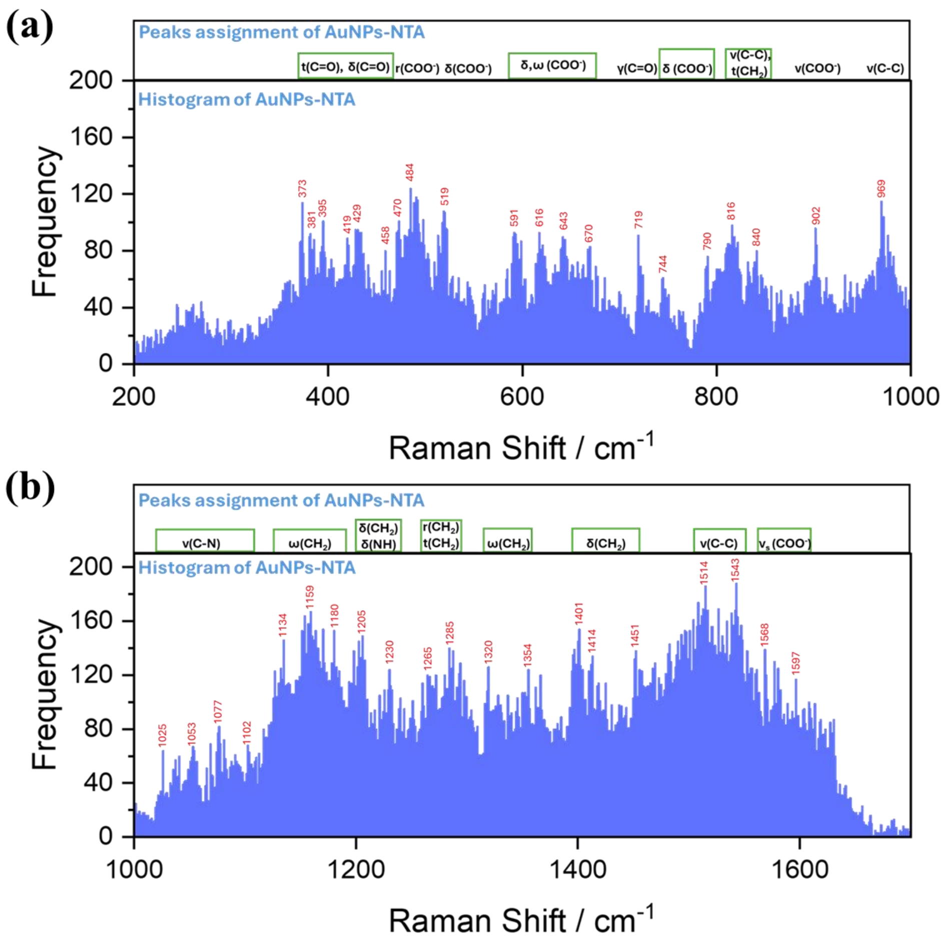


**Figure S11.** Distribution histograms and peaks assignments of the occurrence frequency for Au-NTA during 200-1000 $cm^{-1}$ (a) and 1000-1700 $cm^{-1}$ (b).

## 2. Supplementary Tables

**Table S1. The bands assignments of normal Raman spectrum of NTA powder and SERS spectrum of Au-NTA.**

| Normal Raman of NTA powder (Peak position/ $cm^{-1}$) | SERS of Au-NTA (Peak position/ $cm^{-1}$) | Distribution histograms of the peak's frequency for Au-NTA (Peak position/ $cm^{-1}$) | Assignments | References |
|---|---|---|---|---|
| | | 373, 381,395, 419, 429, 458 | t(CO), δ(C=O) | (1) |
| | | 470, 484 | r(COOH) | (2) |
| | | 519 | δ(COOH) | (5) |
| | | 591 | ω(COOH) | (2) |
| 629 | 629 | 616, 643 | δ(COOH) | (3) |
| | | 670 | δ, ω(COOH) | (4) |
| 701 | 722 | 719 | γ(C=O), δ(COOH) | (5, 6) |
| | | 744, 790 | δ(COOH) | (3, 4) |
| 858 | 821 | 816, 840 | v(C-C), t($CH_2$) | (4) |
| | | 902 | v(C-COOH) | (3, 4) |
| | | 969 | v(C-C) | (4) |
| 1093 | 992 | 1025, 1053, 1077, 1102 | v(C-N) | (4, 6) |
| 1182 | 1133 | 1134, 1159, 1180 | ω($CH_2$) | (4) |
| | 1208 | 1205, 1230 | δ($CH_2$), δ(NH) | (4) |
| 1286 | | 1265, 1285 | r($CH_2$), t($CH_2$) | (4) |
| | | 1320, 1354 | ω($CH_2$) | (4) |
| 1446 | 1420 | 1401, 1414, 1451 | δ($CH_2$) | (4) |
| | | 1514, 1543 | v(C-C) | (6) |
| | | 1568, 1597 | Vs (COOH) | (3) |
| 1611 | | | r($NH_2$), v(COOH) | (3) |
| 1722 | | | v(C=O) | (7) |

**Table S2. The bands assignments of Au-NTA-Ni-Pro and Au-NTA-Ni-Hyp.**

| Single spectrum of Au-NTA-Ni-Pro (Peak position/ $cm^{-1}$) | Single spectrum of Au-NTA-Ni-Hyp (Peak position/ $cm^{-1}$) | Distribution histograms of the peak's frequency for Au-NTA-Ni-Pro (Peak position/ $cm^{-1}$) | Distribution histograms of the peak's frequency for Au-NTA-Ni-Hyp (Peak position/ $cm^{-1}$) | Assignments | References |
|---|---|---|---|---|---|
| | | 256, 270 | 265 | δ(CC=O), r(CCC) | (5) |
| | | 286 | 285 | Ni-O | (8) |
| 411 | 451 | 349, 380, 411 | 340, 384, 405, 440 | Ring bending | (8) |
| 488 | | 455, 485 | 453, 473, 487 | Ring vibration | (8) |
| | | 511, 530 | 531 | δ(CCN) | (4) |
| | | 570 | 567 | p(C=O) | (4) |
| | | 602 | | ω(COOH) | (2) |
| 618, 648 | | 618 | 626 | Ring bending | (8) |
| | | 630, 649 | 642 | r, δ, ω (COOH) | (4) |
| | 695 | 675 | 666 | δ, ω(COOH) | (6) |
| | | 730 | 713, 731 | γ(C=O) | (5, 6) |
| 809 | | 793, 805 | 798 | δ(COOH) | (4) |
| 865 | | 825 | 823, 836 | Ring v(C-C), t($CH_2$) | (4) |
| 919 | | 913 | | v(C-COOH) | (3, 4) |
| | | 935 | 936 | Ring stretching | (8) |
| | | 973 | 960, 972 | v(C-C) | (4) |
| | 991 | 1087 | | v(C-N) | (4, 6) |
| | 1151 | 1150, 1180, 1192 | 1128, 1146, | ω($CH_2$) | (4, 8) |
| | | | 1169 | OH bending | (8) |
| 1225 | | 1233, 1247 | 1210, 1245 | Pro/Hyp ring δ($CH_2$), δ($NH_2$) | (4) |
| | | 1290 | 1288 | r(CH), r(NH) | (8) |
| | 1322 | 1320, 1342 | 1327, 1342, 1367 | ω($CH_2$) | (4) |
| | 1390 | 1398 | 1406 | Vs (COOH) | (1) |
| 1482 | 1450 | 1414, 1432, 1475, 1486 | 1443, 1476, 1489 | δ($CH_2$) | (4) |
| | | 1528 | 1515 | v(C-C) | (6) |
| | | 1558, 1583 | 1557, 1579, 1596 | Vs (COOH) | (3) |
| | | | 1611 | r($NH_2$), v(COOH) | (3) |

# References


(1) Podstawka, E.; Ozaki, Y.; Praniewicz, L.M. *Appl. Spectrosc.* **2005**, *59*, 1516–1526.

(2) Herlinger, A.W.; Long II, T.V. *J. Am. Chem. Soc.* **1970**, *4*, 6481–6486.

(3) Huang, J.A.; Mousavi, M.Z.; Giovannini, G.; Zhao, Y.Q.; Hubarevich, A.; Soler, M.A.; Rocchia, W.; Garoli, D.; Angelis, F.D. *Angew. Chem. Int. Ed.* **2020**, *59*, 11423–11431.

(4) Cárcamo, J.J.; Aliaga, A.E.; Clavijo, E.; Garrido, C.; Gómez–Jeriaand, J. S.; Campos–Vallette, M.M. *J. Raman Spectrosc.* **2012**, *43*, 750–755.

(5) Suzuki, T.; Takahashi, K.; Uehara, H.; Yamanobe, T. J. *Therm. Anal. Calorim.* **2013**, *113*, 1543–1549.

(6) Hernández, B.; Coïc, Y.M.; Pflüger, F.; Kruglik, S.G.; Ghomi, M. *J. Raman Spectrosc.* **2016**, *47*, 210–220.

(7) Bazylewski, P.; Divigalpitiya, R.; Fanchini, G. *RSC Adv.* **2017**, *7*, 2964–2970.

(8) Guerrero, A.R.; Aroca, R.F. *J. Raman Spectrosc.* **2012**, *43*, 478–481.
